# Supplementary material for: Approaching the Basis Set Limit in Gaussian-Orbital-Based Periodic Calculations with Transferability: Performance of Pure Density Functionals for Simple Semiconductors
Source: arXiv:2108.12972 ancillary file (2021-10-08)
Supplement: Supplementary file 1 [file supporting_information.pdf]

# Supplementary Material: Approaching the Basis Set Limit in Gaussian-Orbital-Based Periodic Calculations with Transferability: Performance of Pure Density Functionals for Simple Semiconductors

Joonho Lee,<sup>\*,†</sup> Xintian Feng,<sup>‡</sup> Leonardo A. Cunha,<sup>¶</sup> Jérôme F. Gonthier,<sup>¶</sup>  
Evgeny Epifanovsky,<sup>‡</sup> and Martin Head-Gordon<sup>¶</sup>

<sup>†</sup>*Department of Chemistry, Columbia University, New York, NY, USA*

<sup>‡</sup>*Q-Chem Inc., Pleasanton, CA, USA*

<sup>¶</sup>*Department of Chemistry, University of California, Berkeley, CA, USA*

E-mail: jl5653@columbia.edu

## Sensitivity of pseudopotentials

We confirm the sensitivity of our numerical results with respect to the choice of GTH pseudopotentials. Specifically, we test the band gap performance of BLYP functional with GTH-LDA, GTH-PBE, and GTH-BLYP pseudopotentials using the unc-def2-QZVP basis.

Table S1: The deviation of BLYP band gaps (eV) from experimental values over 43 solids. N/A means “not available”. RMSD, MAD, and MAX denote, respectively, root-mean-square-deviation, mean-average-deviation, and maximum deviation.

|      | GTH-LDA | GTH-PBE | GTH-BLYP |
|------|---------|---------|----------|
| C    | -0.88   | -1.05   | -1.00    |
| Si   | -0.23   | -0.31   | -0.33    |
| Ge   | -0.74   | -0.72   | -0.65    |
| SiC  | -0.57   | -0.70   | -0.67    |
| BN   | -1.19   | -1.36   | -1.32    |
| BP   | -0.74   | -0.86   | -0.85    |
| BAs  | 0.14    | -0.02   | 0.00     |
| BSb  | N/A     | N/A     | N/A      |
| AlP  | -0.53   | -0.61   | -0.63    |
| AlAs | -0.34   | -0.49   | -0.48    |
| AlSb | -0.11   | -0.22   | -0.21    |
| bGaN | -1.44   | -1.61   | -1.58    |
| GaP  | -0.65   | -0.67   | -0.71    |
| GaAs | -1.08   | -1.11   | -1.14    |
| GaSb | -0.65   | -0.73   | -0.73    |
| InP  | -0.85   | -0.80   | -0.87    |
| InAs | -0.41   | -0.41   | -0.41    |
| InSb | -0.23   | -0.23   | -0.23    |
| ZnS  | -1.51   | -1.55   | -1.61    |
| ZnSe | -1.35   | -1.43   | -1.48    |
| ZnTe | -1.00   | -1.12   | -1.17    |
| CdS  | -1.39   | -1.39   | N/A      |
| CdSe | -1.24   | -1.27   | N/A      |
| CdTe | -1.11   | -1.16   | N/A      |
| MgS  | -1.69   | -1.70   | -1.72    |
| MgTe | -0.88   | -0.98   | -0.97    |
| MgO  | -2.05   | -2.22   | -2.18    |
| MgSe | -0.37   | -0.54   | -0.54    |
| CaS  | N/A     | N/A     | N/A      |
| CaSe | N/A     | N/A     | N/A      |
| CaTe | N/A     | N/A     | N/A      |
| SrS  | N/A     | N/A     | N/A      |
| SrSe | N/A     | N/A     | N/A      |
| SrTe | N/A     | N/A     | N/A      |
| BaS  | -1.52   | -1.56   | -1.58    |
| BaSe | -1.39   | -1.48   | -1.49    |
| BaTe | -1.21   | -1.34   | -1.34    |
| LiH  | -1.46   | -1.46   | -1.46    |
| LiF  | -4.71   | -4.86   | -4.84    |
| LiCl | -2.84   | -2.87   | -2.89    |
| AlN  | -1.47   | -1.59   | -1.56    |
| GaN  | -1.38   | -1.56   | -1.53    |
| InN  | -0.69   | -0.69   | -0.69    |
| RMSD | 1.39    | 1.46    | 1.47     |
| MEAN | -1.10   | -1.19   | -1.18    |
